# Supplementary material for: Efficient quantum state preparation through seniority driven operator selection
Source: arXiv:2504.19760 source file (2025-04-28)
Supplement: Supplementary file 1 [file si.tex]

\documentclass[%
aip,jcp,amsmath,amssymb, reprint, linenumbers
]{revtex4-2}
\usepackage{graphicx}
\usepackage{dcolumn}
\usepackage{bm}
\usepackage{amssymb}
\usepackage{amsmath}
\usepackage{supertabular}
\usepackage[table,x11names]{xcolor}
\usepackage{longtable}
\usepackage{colortbl}
\usepackage{multirow}\usepackage{braket}
\usepackage{esvect}
\usepackage{gensymb}
\usepackage{soul}
\let\oldAA\AA
\renewcommand{\AA}{\text{\normalfont\oldAA}}

\usepackage{qtree}
\usepackage{tipa}
\usepackage{appendix}
\usepackage{ulem}
\usepackage{xcolor}
\usepackage{tabularx,booktabs}
\usepackage{simplewick}
\usepackage{simpler-wick}
\usepackage{multirow, makecell}
\usepackage{scalerel}
\usepackage[framemethod=tikz]{mdframed}
\usepackage{mathrsfs}
\usepackage[colorinlistoftodos]{todonotes}
\presetkeys{todonotes}{inline,backgroundcolor=white}{}

\begin{document}
\end{document}
